# Supplementary material for: RED: Robust Environmental Design
Source: arXiv:2411.17026 source file (2024-11-26)
Supplement: Supplementary file 1 [file appendix.tex]

\textcolor{red}{These aglorihms are good, but can you also give a plain English version. Don't get ride of these algorithms, but give a second version that is more plain english.}

\begin{table}[tbh]
  
  \label{tab:lisa_results_appendix}
  \centering
  \resizebox{\textwidth}{!}{%
  \begin{tabular}{lcccccc}
    \toprule
    \textbf{Method} & \textbf{Clean} & \textbf{Sticker Attack} & \textbf{Patch Attack (5\%)} & \textbf{Patch Attack (10\%)} & \textbf{Patch Attack (20\%)} & \textbf{Patch Attack (30\%)} \\ \midrule
    \textbf{LISA} & & & & & \\
    (De)Randomized Smoothing   & 0.82 & 0.68 & 0.80 & 0.76 & 0.75 & 0.67 \\ 
    Full Image       & 1.00 & 0.10 & 0.15 & 0.05 & 0.10 & 0.10 \\ \midrule
    \textbf{GTSRB} & & & & & \\
    (De)Randomized Smoothing  & 0.96 & 0.75 & 0.83 & 0.92 & 0.90 & 0.87 \\ 
    Full Image      & 1.00 & 0.2 & 0.22 & 0.15 & 0.08 & 0.02 \\ \bottomrule
  \end{tabular}
  }
  \caption{Prediction accuracy on LISA GTSRB \textcolor{red}{put your method in here, just one extra row per dataset}
  \textcolor{red}{Need to change this table }}
  
\end{table}

\begin{algorithm}
\caption{Training Algorithm}
\label{alg:train}
\begin{algorithmic}[1]
\State \textbf{Input:} Dataset \(X, Y\), ablation algorithm \(g\).
\State \textbf{Output:} Trained robust road sign backgrounds \(\boldsymbol{\alpha}\) for each class; \(\boldsymbol{\alpha} = \{\alpha_1, \cdots, \alpha_j, \ldots \alpha_m \}\)

\State Initialize \(\alpha_j\) for each road sign class \(j\);

\For{epoch in num\_epochs}
    \State Get the set of ablated images via $g$.
    \State \(l = \sum_{i=1} \sum_{x\in S_i(\alpha)} L(f(s),y_i)\)
    \State \(l.backward()\)
    \If{epoch < 5}
        \State Update \(f\) and \(\boldsymbol{\alpha}\) (warm-up phase)
    \ElsIf{epoch \% 10 == 0}
        \State Update \(f\) and \(\boldsymbol{\alpha}\)
    \Else
        \State Update only \(\boldsymbol{\alpha}\)
    \EndIf
\EndFor
\State \textbf{Return} \(\boldsymbol{\alpha}\)
\end{algorithmic}
\end{algorithm}

\begin{algorithm}
\caption{Ablated Images Set Collection}
\label{alg:ablated_images}
\begin{algorithmic}[1]
\State \textbf{Input:} Image $X'$, patch size $a$, classification model $f$.
\State \textbf{Output:} Set of ablated images $S$.
\State Initialize $S = []$, $W, H = \text{dimensions of } X'$ 
\For{$i = 0$ to $\frac{W}{a} - 1$}
    \For{$j = 0$ to $\frac{H}{a} - 1$}
        \State Create mask with ones at $[i \cdot a:(i+1) \cdot a, j \cdot a:(j+1) \cdot a]$ and zeros elsewhere
        \State $s = \text{mask} \times X'$  % Element-wise multiplication
        \State Append $s$ to $S$
    \EndFor
\EndFor
\State \textbf{Return} $S$
\end{algorithmic}
\end{algorithm}

\begin{algorithm}
\caption{Majority Vote Inference Algorithm}
\label{alg:majority_vote}
\begin{algorithmic}[1]
\State \textbf{Input:} Image $X'$, mask size $a$, model $f$.
\State \textbf{Output:} Prediction for $X'$.
\State $S \leftarrow$ Set of ablated images from Algorithm \ref{alg:ablated_images}.
\State Initialize $P = []$.
\For{each $s$ in $S$}
    \State $P \leftarrow P \cup \{f(s)\}$  % Append model prediction for each patch
\EndFor
\State $y_p \leftarrow \text{majority\_vote}(P)$  % Compute majority vote from predictions
\State \textbf{Return} $y_p$
\end{algorithmic}
\end{algorithm}

\begin{figure}[h]
\centering
\includegraphics[width=0.95\textwidth]{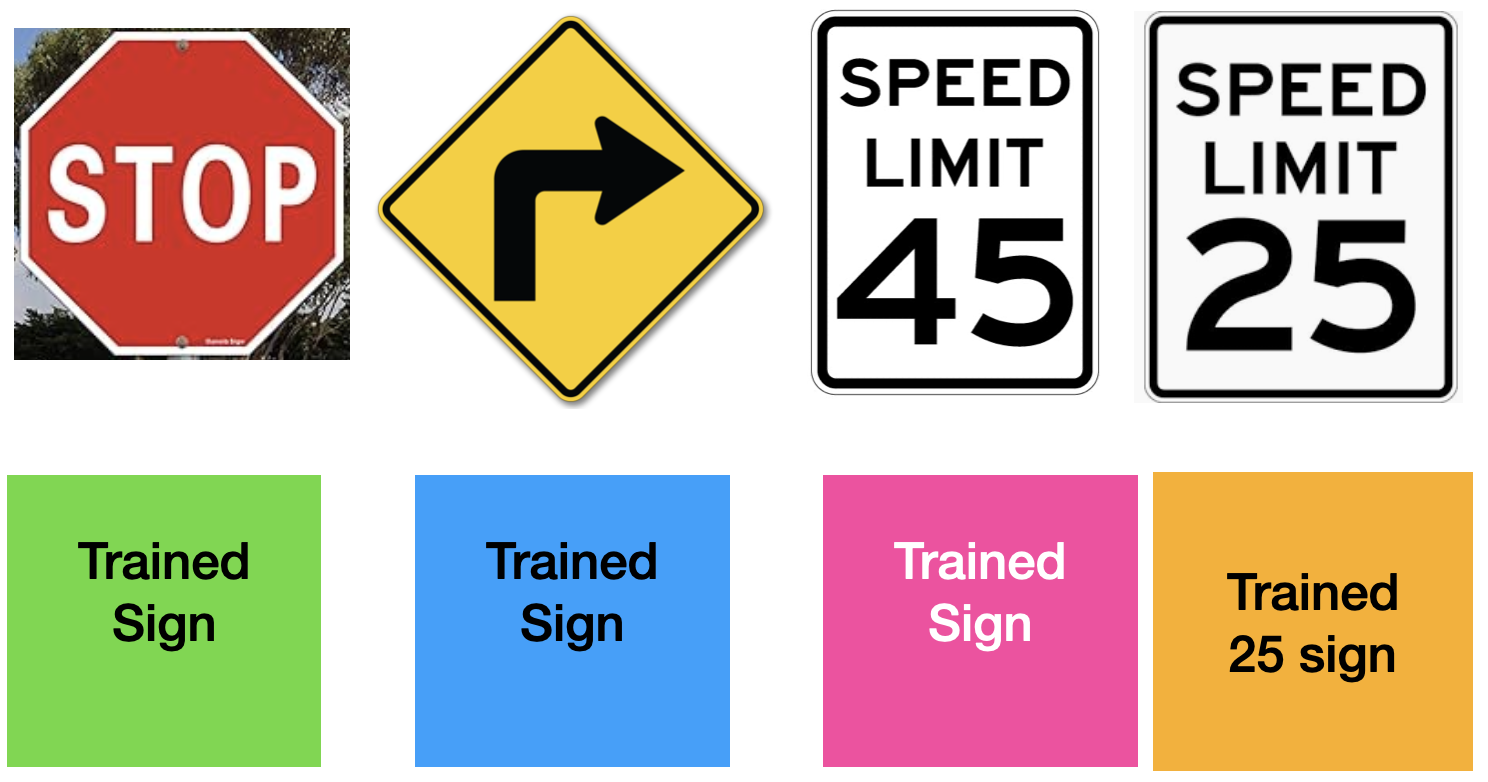}
\caption{\todo{This figure will go to appendix}}
\label{fig:different_signs}
\end{figure}
